# Supplementary material for: Disentangling Video with Independent Prediction
Source: arXiv:1901.05590 source file (2019-01-17)
Supplement: Supplementary file 1 [file appendix.tex]

\newpage

\appendix

\section*{Appendix A}\label{appendix-a}
\addcontentsline{toc}{section}{Appendix A}
